# Supplementary material for: Enough?
Source: arXiv:2501.12161 source file (2025-01-21)
Supplement: Supplementary file 1 [file appendix.tex]

\section{Appendix}
